# Supplementary material for: Weakly supervised cross-domain alignment with optimal transport
Source: arXiv:2008.06597 source file (2020-08-14)
Supplement: Supplementary file 1 [file Ablation_sm.tex]

\begin{table*}[h!] \footnotesize
    \begin{center}
    % \begin{tabular}{lccccccc}
        \caption{Ablation study on Flickr30K. In the first section, we try to use adaptive features. In the second section, we compare the performance of different network architectures for text representations.}
        \label{table:ablation_sm}
            \centering
        \begin{tabular*}{1.\linewidth}{@{\extracolsep{\fill}}lccccccc}
            \toprule
            % \noalign{\smallskip}
             & \multicolumn{3}{c}{Sentence Retrieval} & \multicolumn{3}{c}{Image Retrieval} & \multicolumn{1}{c}{} \\
            Method & R@1 & R@5 & R@10 & R@1 & R@5 & R@10 & Rsum\\
            % \noalign{\smallskip}
            \hline
            \noalign{\smallskip}
            $\cos$ + OT, fixed & 67.4 & 90.3 & 94.9 & 48.2 & 76.7 & {84.8} &462.3 \\ 
            $\cos$ + OT, adaptive & 64.8 & 88.3 &94.5 & 45.9 & 74.5 & 83.5 &451.5 \\
            % \midrule
            % $\cos$, $\eta$=0.2  & 61.7 & 87.4 & 93.5 & 48.5 & 76.0 & 83.7 & 450.8 \\ 
            % $\cos$ + OT, $\eta$=0.2, $\lambda$=1 & 66.2 & 89.0 & 94.1 & 48.9 & 77.5 & {85.4} &461.1 \\ 
            % % \hline
            % $\cos$, $\eta$=0.12  & 63.1 &89.5 & 94.3 & {50.5} & 77.1 & 84.7&459.2 \\ 
            % $\cos$ + OT, $\eta$=0.12, $\lambda$=2 & {69.3} & {91.0} &{95.7} & 48.4 & {77.2} & 84.7 &{466.3} \\
            \midrule
            $\cos$+OT, bi-GRU &{67.9} &{91.0} &{94.9} &{49.8} &{77.5} &{85.2} &{466.3}\\
            $\cos$+OT, Transformer, 1 layer, 8 heads & 57.8 & 86.8 & 93.1 & 46.4 & 74.4 & {82.9} &441.4 \\ 
            $\cos$+OT, Transformer, 2 layer, 8 heads  & 44.1 & 74.8 &84.1 & 31.7 & 62.7 & 73.5 &370.9 \\
            \midrule
            PFAN & 66 & 89.6 & 94.3 & 49.6 & 77 & 84.2 & 460.7 \\
            PFAN + OT & 67.1 & 89.2 & 94.3 & 50 & 78 & 85.7 & 464.3\\
            SCAN & 46.4 & 77.4 & 87.2 & 34.4 & 63.7 & 75.7 & 384.8 \\
            SCAN + OT & 50.1 & 80.1 & 89.3 & 37.9 & 66.9 & 78.2 & 402.5 \\ 
            \bottomrule
        \end{tabular*}
    \end{center}
    % \vspace{-5mm}
\end{table*}
