# Supplementary material for: Weakly supervised cross-domain alignment with optimal transport
Source: arXiv:2008.06597 source file (2020-08-14)
Supplement: Supplementary file 2 [file SM_vqa.tex]

\begin{table}[h!]\small
    \begin{center}
    \caption{%\footnotesize 
  VQA validation dataset results
    }
    %   \vspace{-3mm}
    \label{table:sm_vqa}
    \centering
      % \begin{tabular}{lccccccc}
    %   \begin{tabular}{1.\textwidth}{@{\extracolsep{\fill}}lccc}
        \begin{tabular}{lc}
           \toprule
          %  \noalign{\smallskip}
        %    & \multicolumn{3}{c}{Sentence Retrieval} & \multicolumn{3}{c}{Image Retrieval} & \multicolumn{1}{c}{}\\
          Method & VQA-score\\
          % \noalign{\smallskip}
          \toprule
          % \noalign{\smallskip}
          % & \multicolumn{7}{c}{Flickr30K} \\ 
          % \hline
          % \noalign{\smallskip}
          BAN~\cite{kim2018bilinear} & 66.06   \\
          Ours & 66.20  \\
        %   OT\_S & 25.54 & 58.05 & 69.62 \\
            \bottomrule
      \end{tabular}
  
      \vspace{-8mm}
    \end{center}
  \end{table}
